# Supplementary material for: Programmable electrical coupling between stochastic magnetic tunnel junctions
Source: arXiv:2312.13171 source file (2023-12-20)
Supplement: Supplementary file 1 [file old_appendices.tex]

\section{\label{sec:Circuit_details}Circuit Details}

This section contains technical details about each amplifier stage in our coupling circuit. There are two inversions on each side of the loop due to the gain stage and the transconductance stage, and an additional inversion can be added to get negative coupling by swapping the op-amp terminals in the threshold stage. All amplifiers are AD820 op-amps.\footnote{{Certain commercial components are identified in this paper to foster understanding. Such identification does not imply recommendation or endorsement by the National Institute of Standards and Technology, nor does it imply that the processes and software identified are necessarily the best available for the purpose.}} In addition to the amplifier stages discussed in the following sections, the circuit also features a slow-turn-on feature and a debugging mode. The slow turn on feature is an RC circuit that slowly applies the desired current to the SMTJ connected to the board to avoid destroying the tunnel barrier. The debugging mode allows us to use a function generator as the input signal on one side of the loop rather than an SMTJ. 

\subsection{Threshold Stage}

\begin{figure}
    \centering
    \includegraphics[width=6.5cm]{figures/threshold_circuit.drawio.pdf}
    \caption{Threshold stage circuit schematic. $I_{fixed}$ is 1~mA and $R_{var}$ is a 1~k$\Omega$ digital potentiometer. This allows us to set the digitization threshold voltage between 0~V and 1~V, which covers the range of switching of our SMTJs.}
    \label{fig:threshold-stage}
\end{figure}

The threshold stage shown in Fig.~\ref{fig:threshold-stage} converts an analog input voltage $V_{in}$ into a digital output voltage $V_{out}$. If $V_{in}$ is above some reference voltage, the output will be high, otherwise it will be low. It consists of an op-amp, a fixed current source, and a variable resistor. The current source and variable resistor together set the digitization reference voltage. The transfer function for the threshold stage is
\begin{equation}
    V_{out} = 
    \begin{cases} 
      0~V & V_{in}\leq I_{fixed}*R_{var} \\
      2.5~V & otherwise\\
   \end{cases}.
\end{equation}
This transfer function is for the positive coupling case, but on our circuit, we have implemented a switch that allows us to change the polarity of the interaction by switching the op-amp inputs. This way, we can have both positive and negative coupling on the same board. 

It should be emphasized that the comparison is done by an op-amp without feedback rather than a digital comparator. Our op-amps are general purpose and have a 1.8~MHz gain-bandwidth product, making them non-ideal for high-speed applications. 

\subsection{Gain Stage}

\begin{figure}
    \centering
    \includegraphics[width=7cm]{figures/gain_stage_circuit.drawio.pdf}
    \caption{Gain stage circuit schematic. $R_1$ is a 100~k$\Omega$ fixed resistor, and $R_{var}$ is a 10~k$\Omega$ digital potentiometer. This makes the gain variable between 0 and 0.1. The output signal is centered at $V_c$ = 1.25~V.}
    \label{fig:gain-stage}
\end{figure}

The gain stage circuit shown in Fig.~\ref{fig:gain-stage} adjusts the voltage difference between high and low levels of the digital output from the threshold stage while keeping it centered at the voltage $V_c$. The voltage difference is proportional to the gain, which is set by $R_{var}$. The transfer function for this stage is
\begin{equation}
    V_{out} = G(V_c - V_{in}) + V_c,
\end{equation}
where $G = R_{var}/R_1$ is the gain. This configuration is inverting: the output changes in the opposite direction as the input.

\subsection{Level Shifting Stage}

\begin{figure}
    \centering
    \includegraphics[width=7cm]{figures/level_shifting_circuit.drawio.pdf}
    \caption{Level shifting stage circuit schematic. In our circuit, $R_1 = R_f = R_2 = R_g = 10~k\Omega$. The output voltage is the input voltage shifted by $V_{bias}$, which is adjusted through digital potentiometers.}
    \label{fig:level-shift-stage}
\end{figure}

The level shifting stage shown in Fig.~\ref{fig:level-shift-stage} takes the scaled gain stage output and shifts the center to a different DC voltage. The transfer function is written as
\begin{equation}
    V_{out} = \frac{(R_1 + R_f)R_g}{(R_2 + R_g)R_1}V_{in} + \frac{(R_1 + R_f)R_2}{(R_2 + R_g)R_1}V_{bias}.
\end{equation}
Taking $R_1 = R_2 = R_g = R_f$, as it is in our circuit, the expression for $V_{out}$ simplifies to
\begin{equation}
    V_{out} = V_{in} + V_{bias}
\end{equation}
This configuration is noninverting. The new center voltage can be adjusted by changing $V_{bias}$. The method for adjusting $V_{bias}$ is similar to the way we set the threshold stage reference voltage in Fig.~\ref{fig:threshold-stage}: with a fixed current source connected to two digital potentiometers of different resolutions. 

% Using the transfer functions from each stage, the change in current levels due to an increment in gain can be determined. \textcolor{red}{derive $\Delta I$ with respect to gain}

\subsection{Transconductance Stage}

\begin{figure}
    \centering
    \includegraphics[width=5cm]{figures/transconductance_circuit.drawio.pdf}
    \caption{Transconductance stage circuit schematic. $V_{dd}$ is 15~V and $R_1$ is 10~$k\Omega$. This circuit converts an input voltage to a proportional output current.}
    \label{fig:transconductance-stage}
\end{figure}

The transconductance stage shown in Fig.~\ref{fig:transconductance-stage} converts the shifted digital signal from the level shifting stage into a proportional current. The transfer function that describes this relationship is 
\begin{equation}
    I_{out} = \frac{V_{dd} - V_{in}}{R_1}
\end{equation}
This configuration is inverting. This output current will be digital, with two discrete levels that move farther apart as $R_{var}$ in the gain stage increases. If this gain stage $R_{var}$ is set to 0~$\Omega$, the difference $2\Delta I$ between discrete current levels is 0~A and the transconductance stage output is a DC current. The adjustable $V_{bias}$ in the level shifting stage allows us to set this DC current. In this way, we can bias the SMTJs to 50~\% or to any point that we choose. The relationship between output current and gain can be derived analytically using these transfer functions.

\appendix

% \section{\label{sec:Circuit_details}Circuit Details}

% This section contains technical details about each amplifier stage in our coupling circuit. There are two inversions on each side of the loop due to the gain stage and the transconductance stage, and an additional inversion can be added to get negative coupling by swapping the op-amp terminals in the threshold stage. All amplifiers are AD820 op-amps.\footnote{{Certain commercial components are identified in this paper to foster understanding. Such identification does not imply recommendation or endorsement by the National Institute of Standards and Technology, nor does it imply that the processes and software identified are necessarily the best available for the purpose.}} In addition to the amplifier stages discussed in the following sections, the circuit also features a slow-turn-on feature and a debugging mode. The slow turn on feature is an RC circuit that slowly applies the desired current to the SMTJ connected to the board to avoid destroying the tunnel barrier. The debugging mode allows us to use a function generator as the input signal on one side of the loop rather than an SMTJ. 

% \subsection{Threshold Stage}

% \begin{figure}
%     \centering
%     \includegraphics[width=6.5cm]{figures/threshold_circuit.drawio.pdf}
%     \caption{Threshold stage circuit schematic. $I_{fixed}$ is 1~mA and $R_{var}$ is a 1~k$\Omega$ digital potentiometer. This allows us to set the digitization threshold voltage between 0~V and 1~V, which covers the range of switching of our SMTJs.}
%     \label{fig:threshold-stage}
% \end{figure}

% The threshold stage shown in Fig.~\ref{fig:threshold-stage} converts an analog input voltage $V_{in}$ into a digital output voltage $V_{out}$. If $V_{in}$ is above some reference voltage, the output will be high, otherwise it will be low. It consists of an op-amp, a fixed current source, and a variable resistor. The current source and variable resistor together set the digitization reference voltage. The transfer function for the threshold stage is
% \begin{equation}
%     V_{out} = 
%     \begin{cases} 
%       0~V & V_{in}\leq I_{fixed}*R_{var} \\
%       2.5~V & otherwise\\
%    \end{cases}.
% \end{equation}
% This transfer function is for the positive coupling case, but on our circuit, we have implemented a switch that allows us to change the polarity of the interaction by switching the op-amp inputs. This way, we can have both positive and negative coupling on the same board. 

% It should be emphasized that the comparison is done by an op-amp without feedback rather than a digital comparator. Our op-amps are general purpose and have a 1.8~MHz gain-bandwidth product, making them non-ideal for high-speed applications. 

% \subsection{Gain Stage}

% \begin{figure}
%     \centering
%     \includegraphics[width=7cm]{figures/gain_stage_circuit.drawio.pdf}
%     \caption{Gain stage circuit schematic. $R_1$ is a 100~k$\Omega$ fixed resistor, and $R_{var}$ is a 10~k$\Omega$ digital potentiometer. This makes the gain variable between 0 and 0.1. The output signal is centered at $V_c$ = 1.25~V.}
%     \label{fig:gain-stage}
% \end{figure}

% The gain stage circuit shown in Fig.~\ref{fig:gain-stage} adjusts the voltage difference between high and low levels of the digital output from the threshold stage while keeping it centered at the voltage $V_c$. The voltage difference is proportional to the gain, which is set by $R_{var}$. The transfer function for this stage is
% \begin{equation}
%     V_{out} = G(V_c - V_{in}) + V_c,
% \end{equation}
% where $G = R_{var}/R_1$ is the gain. This configuration is inverting: the output changes in the opposite direction as the input.

% \subsection{Level Shifting Stage}

% \begin{figure}
%     \centering
%     \includegraphics[width=7cm]{figures/level_shifting_circuit.drawio.pdf}
%     \caption{Level shifting stage circuit schematic. In our circuit, $R_1 = R_f = R_2 = R_g = 10~k\Omega$. The output voltage is the input voltage shifted by $V_{bias}$, which is adjusted through digital potentiometers.}
%     \label{fig:level-shift-stage}
% \end{figure}

% The level shifting stage shown in Fig.~\ref{fig:level-shift-stage} takes the scaled gain stage output and shifts the center to a different DC voltage. The transfer function is written as
% \begin{equation}
%     V_{out} = \frac{(R_1 + R_f)R_g}{(R_2 + R_g)R_1}V_{in} + \frac{(R_1 + R_f)R_2}{(R_2 + R_g)R_1}V_{bias}.
% \end{equation}
% Taking $R_1 = R_2 = R_g = R_f$, as it is in our circuit, the expression for $V_{out}$ simplifies to
% \begin{equation}
%     V_{out} = V_{in} + V_{bias}
% \end{equation}
% This configuration is noninverting. The new center voltage can be adjusted by changing $V_{bias}$. The method for adjusting $V_{bias}$ is similar to the way we set the threshold stage reference voltage in Fig.~\ref{fig:threshold-stage}: with a fixed current source connected to two digital potentiometers of different resolutions. 

% % Using the transfer functions from each stage, the change in current levels due to an increment in gain can be determined. \textcolor{red}{derive $\Delta I$ with respect to gain}

% \subsection{Transconductance Stage}

% \begin{figure}
%     \centering
%     \includegraphics[width=5cm]{figures/transconductance_circuit.drawio.pdf}
%     \caption{Transconductance stage circuit schematic. $V_{dd}$ is 15~V and $R_1$ is 10~$k\Omega$. This circuit converts an input voltage to a proportional output current.}
%     \label{fig:transconductance-stage}
% \end{figure}

% The transconductance stage shown in Fig.~\ref{fig:transconductance-stage} converts the shifted digital signal from the level shifting stage into a proportional current. The transfer function that describes this relationship is 
% \begin{equation}
%     I_{out} = \frac{V_{dd} - V_{in}}{R_1}
% \end{equation}
% This configuration is inverting. This output current will be digital, with two discrete levels that move farther apart as $R_{var}$ in the gain stage increases. If this gain stage $R_{var}$ is set to 0~$\Omega$, the difference $2\Delta I$ between discrete current levels is 0~A and the transconductance stage output is a DC current. The adjustable $V_{bias}$ in the level shifting stage allows us to set this DC current. In this way, we can bias the SMTJs to 50~\% or to any point that we choose. The relationship between output current and gain can be derived analytically using these transfer functions.

% \section{\label{sec:Wobbliness}Device Non-Idealities}

% \begin{figure}
%     \centering
%     \includegraphics[width=8cm]{figures/Wobble_Test.pdf}
%     \caption{(a) Statistical variation in SMTJ AP state probability over 20 trials. (b) Statistical variation in mean dwell time over 20 trials. Each trial is averaged over 10 million points, equivalent to roughly 8000 switches. Trials were done sequentially with a 30 second delay between trials.}
%     \label{fig:wobbly-test}
% \end{figure}

% \begin{figure}
%     \centering
%     \includegraphics[width=8cm]{figures/Noninverting_Identical_Joint_Probability.pdf}
%     \caption{Probability of joint states during positive coupling experiment with SMTJ-1 and SMTJ-2, which have similar switching time scales. The SMTJs used in this work exhibit unstable behavior that causes unreliable statistics. This explains the large variation in probability despite averaging over a sufficient amount of data.}
%     \label{fig:wobbly-probability}
% \end{figure}

% While performing our experiments, we encountered some difficulty setting the SMTJs to a fixed probability of being in either state. Figure~\ref{fig:wobbly-test} displays the results from a test that was conducted to investigate this effect. A fixed current flows through the device, and 10 million points (8000 switches) of data were collected every 30 seconds. The probability calculation is simply the amount of time spent in the AP state divided by the total time. Changing the number of switches had no obvious effect on the probability variation across trials, nor did changing the amount of time between trials. This indicates that the variation is likely to be intrinsic to the devices rather than due to temperature, inaccurate statistics, or other factors related to the experimental setup.

% There are several possible explanations for this variation in probability. One is that our experiments are done without an applied magnetic field, necessitating the use of high currents that are very close to the breakdown current. This can cause fluctuations in the device's resistance. Another is the presence of defects in the SMTJs. It is possible that some parts of the magnetic domain are not switching coherently with the rest of the domain. There is also no temperature control in our setup, so some of the instability we observe could be due to self-heating. 

% The effect of this instability on the coupling experiments is largely unnoticeable in the experimental dwell time plots in Section~\ref{sec:Results} (Fig.~\ref{fig:noninv-identical-corr}(b), Fig.~\ref{fig:inv-identical-corr}(b), and Fig.~\ref{fig:noninv-diff-corr}(b)). However, plotting the probability of each joint state as a function of gain during the coupling experiment, as in Fig.~\ref{fig:wobbly-probability}, clearly shows that this effect impacts our experiments. Using these SMTJs, we are unable to guarantee a fixed probability of being in either state, which is an important aspect of probabilistic computing. Although the SMTJs used in these experiments exhibit some non-ideal behavior, the experimental demonstrations of coupling are no less valid. 

% \section{\label{sec:software}Software routines}
% Several software routines were employed to run the experiment and to increase the accuracy of our results. First, the simulated annealing algorithm includes automatic gain control. The gain is set through a digital potentiometer on the PCB that uses the I2C communication protocol. We use PySerial to send the desired potentiometer update to an Arduino, which then converts the request into an I2C signal for the potentiometer. The second piece of software we developed for this experiment is a closed loop feedback technique for setting the SMTJ to 50~\% probability of being in each state. This is run at the beginning of each experiment so there is no bias towards either state, but if initial bias were desired this technique could easily be used to set the SMTJ to any probability. Due to some unstable behavior observed in our devices, even with this technique it was difficult to set the device to a desired probability. A discussion of this observation can be found Appendix \ref{sec:Wobbliness}. The third software technique we developed is automatic sampling rate adjustment with increasing gain. To get a statistically significant number of switches at high gain, sampling must be done over a much longer period of time, making fast sampling impractical and unnecessary. 
